# Supplementary material for: Local and Global Information in Obstacle Detection on Railway Tracks
Source: arXiv:2307.15478 source file (2023-07-28)
Supplement: Supplementary file 1 [file appendixA.tex]

\section{Ablation Study on Patch Size}
\label{sec:results_ablation}

In Table \ref{tab:results_patch}, we show evaluation scores for all methods with different patch sizes $K_p$. It can be seen that \textit{PatchDiff} ($\mathcal{L}_{MSE}$) and \textit{PatchDiff} ($\mathcal{L}_{SSIM}$) perform best at a small patch size of $K_p = 13$, whereas our other methods have a peak at $K_p = 21$. Therefore, we use a this optimal value of $K_p=21$ in our evaluations (Section \ref{sec:results}). With increasing patch sizes, obstacle detection quality decreases gradually. This effect is strong for the reconstruction-based \textit{PatchDiff} methods, and in particular for \textit{PatchDiff} ($\mathcal{L}_{MSE}$) and \textit{PatchDiff} ($\mathcal{L}_{SSIM}$). One potential reason for this is that large patches (e.g. $K_p = 51$) contain a lot of railway regions even if a small obstacle is present. Consequently, from the perspective of a \textit{PatchDiff} model, these patches look more similar to the corresponding generated obstacle-free railway patches than to random image patches. The small difference caused by the obstacle is not weighted enough and the patches are classified as being semantically similar. 

\vspace{3mm}
We grid search over different localization parameters $\theta$ and $K_d$ and report the F1 score of the best combination. An interesting observation from this grid search is that for models with smaller patch sizes $K_p$, the optimal threshold $\theta$ separating obstacle regions from railway regions is very high. It is combined with a small optimal density patch size $K_d$. Models with small patch size $K_p \in \{13, 21\}$ are very confident on obstacles, whereas their main weakness is mis-classification of non-obstacle railway structures such as snow, grass or railway crossings. A high $\theta \geq 0.9$ and small $K_d \leq 11$ shift the focus to small regions with extremely high classification / difference values (often corresponding to obstacles) and limit the effect of large regions with medium classification / difference values (often corresponding to mis-classified railway structures). It is logical that such a combination yields the best localization F1 score. For reconstruction-based \textit{PatchDiff} models with large patch sizes $K_p$ (e.g. $K_p = 51$), however, the situation is different. Models are very confidently classifying standard railway patches as non-obstacle regions (very low classification / difference values). Again, this is probably caused by a lot of similar railway structure being visible in both the original and the reconstructed patches. Unfortunately, \textit{PatchDiff} models with large $K_p$ tend to overlook the weak signals caused by small obstacles, and over-confidently classify such anomalous patches as obstacle-free. As a consequence, the best F1 scores are reached when focusing on large regions with medium classification / difference values (often corresponding to patches with overlooked obstacles) with a small $\theta$ and large $K_d$. 

\begin{table}[h]
\begin{center}
 \caption{Ablation study on patch size $K_p$. We report \ac{AUROC} and the best localization F1 score with corresponding $\theta$ and $K_d$, computed on our \textit{FishyrailsCropped} evaluation dataset. Overall, $K_p=21$ gives the best results.}\vspace{1ex}
 \label{tab:results_patch}
 \begin{tabular}{|lll|c|cc|}
 \hline
 Method & $K_p$ & $\mathcal{L}_{AE}$ & ROC AUC & F1 & ($\theta$, $K_d$) \\ \hline \hline
  DeeplabV3 & - & - & 0.817 & 0.535 & (0.3, 51) \\
 RMSE AE & - & $\mathcal{L}_{MSE}$ & 0.686 & 0.498 & (0.2, 7)\\
 SSIM AE & - & $\mathcal{L}_{SSIM}$ & 0.737 & 0.429 & (0.65, 21)\\ 
 Students17 & - & - & 0.555 & 0.405 & (0.25, 7) \\ 
 Students33 & - & - & 0.594 & 0.458 & (0.2, 35) \\ 
 Students65 & - & - & 0.523 & 0.276 & (0.15, 21) \\ \hline
  PatchClass & 13 & - & 0.921 & 0.836 & (0.95, 7)\\ 
 PatchDiff & 13 & $\mathcal{L}_{MSE}$ & 0.920 & 0.835 & (0.95, 7)\\
 PatchDiff & 13 & $\mathcal{L}_{SSIM}$ & 0.921 & 0.830 & (0.95, 7)\\
 PatchDiff & 13 & $\mathcal{L}_{GAN}$ & 0.924 & 0.837 & (0.95, 7)\\
 PatchDiff & 13 & $\mathcal{L}_{GAN} + \mathcal{L}_{HIST}$ & \textbf{0.931} & \textbf{0.839} & (0.95, 7)\\ \hline
 PatchClass & 21 & - & 0.926 & \underline{\textbf{0.863}} & (0.95, 11)\\
 PatchDiff & 21 & $\mathcal{L}_{MSE}$ & 0.917 & 0.825 & (0.9, 7)\\
 PatchDiff & 21 & $\mathcal{L}_{SSIM}$ & 0.915 & 0.812 & (0.95, 7)\\
 PatchDiff & 21 & $\mathcal{L}_{GAN}$ & 0.935 & 0.857 & (0.95, 11)\\
 PatchDiff & 21 & $\mathcal{L}_{GAN} + \mathcal{L}_{HIST}$ & \underline{\textbf{0.936}} & 0.838 & (0.95, 7)\\ \hline
  PatchClass & 29 & - & 0.928 & \textbf{0.861} & (0.95, 11)\\
 PatchDiff & 29 & $\mathcal{L}_{MSE}$ & 0.906 & 0.802 & (0.35, 21)\\
 PatchDiff & 29 & $\mathcal{L}_{SSIM}$ & 0.907 & 0.795 & (0.35, 35)\\
 PatchDiff & 29 & $\mathcal{L}_{GAN}$ & 0.934 & 0.844 & (0.9, 13)\\
 PatchDiff & 29 & $\mathcal{L}_{GAN} + \mathcal{L}_{HIST}$ & \underline{\textbf{0.936}} & 0.846 & (0.9, 11)\\ \hline
  PatchClass & 35 & - & 0.925 & \textbf{0.839} & (0.95, 11)\\
 PatchDiff & 35 & $\mathcal{L}_{MSE}$ & 0.896 & 0.764 & (0.35, 13)\\
 PatchDiff & 35 & $\mathcal{L}_{SSIM}$ & 0.871 & 0.724 & (0.15, 51)\\
 PatchDiff & 35 & $\mathcal{L}_{GAN}$ & \textbf{0.932} & 0.829 & (0.9, 13)\\
 PatchDiff & 35 & $\mathcal{L}_{GAN} + \mathcal{L}_{HIST}$ & 0.930 & 0.826 & (0.55, 29)\\ \hline
  PatchClass & 51 & - & \textbf{0.927} & \textbf{0.832} & (0.95, 11)\\
 PatchDiff & 51 & $\mathcal{L}_{MSE}$ & 0.824 & 0.625 & (0.05, 51)\\
 PatchDiff & 51 & $\mathcal{L}_{SSIM}$ & 0.815 & 0.622 & (0.05, 51)\\
 PatchDiff & 51 & $\mathcal{L}_{GAN}$ & 0.918 & 0.794 & (0.45, 35)\\
 PatchDiff & 51 & $\mathcal{L}_{GAN} + \mathcal{L}_{HIST}$ & 0.914 & 0.782 & (0.3, 35)\\ \hline
 \end{tabular}
\end{center}
\end{table}
