# Supplementary material for: Local and Global Information in Obstacle Detection on Railway Tracks
Source: arXiv:2307.15478 source file (2023-07-28)
Supplement: Supplementary file 2 [file appendixB.tex]

\section{Implementation}
\label{sec:implementation}

The patch-wise classification network $N$ is implemented as a fully convolutional network with skip connections. 
We empirically determine an optimal patch size of $K_p = 21$. The architecture is shown in the Appendix. 
For network optimization, we use stochastic gradient descent with a batch size of 32, initial learning rate of 0.1, momentum of 0.9, and weight decay of $10^{-4}$. 
We train all models until convergence and decrease the learning rate by a factor of $0.1$ after the 10th, 20th, and 25th epoch. 
From now on, we refer to patch classification models as \textit{PatchClass}.

For our extension, the generator $G$ is implemented as a fully convolutional auto-encoder with bottleneck dimension $d = 392$. 
Its architecture is given in the Appendix. We chose the typical structural similarity patch size $K_s=11$ in $\mathcal{L}_{SSIM}$. 
When computing $\mathcal{L}_{HIST}$, we choose $256$ histogram bins. In total, we train $G$ for 200 epochs with four different loss combinations. 
We use Adam optimization and the hyper-parameters shown in the appendix. When training the discriminator, we apply label smoothing with label smoothing coefficient 0.9 and weight the discriminator loss with 0.5. 
The discriminator's architecture is described in the Appendix as well.

\section{Neural Network Architectures}
\label{sec:architectures}

\begin{table}[h]
\begin{center}
 \caption{Hyper-parameters for training the generator $G$.}\vspace{1ex}
 \label{tab:g_params}
 \begin{tabular}{l|cccc}
  & $\mathcal{L}_{MSE}$ & $\mathcal{L}_{SSIM}$ & $\mathcal{L}_{GAN}$ & $\mathcal{L}_{GAN} + \mathcal{L}_{HIST}$ \\ \hline 
 Batch size & 64 & 64 & 64 & 16 \\
 Generator learning rate & 0.1 & 0.1 & $10^{-4}$ & $10^{-4}$ \\
 Discriminator learning rate & - & - & $10^{-4}$ & $10^{-4}$ \\
 Momentum & 0.9 & 0.9 & 0.5 & 0.5 \\
 Weight decay & $10^{-4}$ & $10^{-4}$ & $10^{-4}$ & $10^{-4}$ \\

 \end{tabular}
\end{center}
\end{table}

\begin{table}[h]
\begin{center}
 \caption{Network architecture for generator $G$. Except for the input and layer 40, each layer is followed by a batch normalization layer and ReLU activation. Layer 40 is followed by a tanh activation layer. TConv2d denotes transposed convolutional layers \cite{Zeiler2010}. }\vspace{1ex}
 \label{tab:g}
 \begin{tabular}{lllcccc}
 No. & Layer & Input & Output Size & Kernel & Stride & Padding \\ \hline 
 0 & Input & $\textbf{x}$ & 224x224x3 & & & \\ 
 1 & Conv2d & 0 & 224x224x32 & 3x3 & 1 & 1 \\
 2 & Conv2d & 1 & 224x224x32 & 3x3 & 1 & 1 \\
 3 & Conv2d & 2 & 112x112x32 & 4x4 & 2 & 1 \\
 4 & Conv2d & 3 & 112x112x32 & 3x3 & 1 & 1 \\
 5 & Conv2d & 4 & 112x112x32 & 3x3 & 1 & 1 \\
 6 & Conv2d & 5 & 56x56x64 & 4x4 & 2 & 1 \\
 7 & Conv2d & 6 & 56x56x64 & 3x3 & 1 & 1 \\
 8 & Conv2d & 7 & 56x56x64 & 3x3 & 1 & 1 \\
 9 & Conv2d & 8 & 28x28x64 & 4x4 & 2 & 1 \\
 10 & Conv2d & 9 & 28x28x64 & 3x3 & 1 & 1 \\
 11 & Conv2d & 10 & 28x28x64 & 3x3 & 1 & 1 \\
 12 & Conv2d & 11 & 14x14x128 & 4x4 & 2 & 1 \\
 13 & Conv2d & 12 & 14x14x128 & 3x3 & 1 & 1 \\
 14 & Conv2d & 13 & 14x14x128 & 3x3 & 1 & 1 \\
 15 & Conv2d & 14 & 7x7x256 & 4x4 & 2 & 1 \\
 16 & Conv2d & 15 & 7x7x128 & 3x3 & 1 & 1 \\
 17 & Conv2d & 16 & 7x7x64 & 3x3 & 1 & 1 \\
 18 & Conv2d & 17 & 7x7x32 & 3x3 & 1 & 1 \\
 19 & Conv2d & 18 & 7x7x32 & 3x3 & 1 & 1 \\
 20 & Conv2d & 19 & 7x7x8 & 3x3 & 1 & 1 \\
 21 & TConv2d & 20 & 7x7x16 & 3x3 & 1 & 1 \\
 22 & TConv2d & 21 & 7x7x32 & 3x3 & 1 & 1 \\
 23 & TConv2d & 22 & 7x7x64 & 3x3 & 1 & 1 \\
 24 & TConv2d & 23 & 7x7x128 & 3x3 & 1 & 1 \\
 25 & TConv2d & 24 & 7x7x256 & 3x3 & 1 & 1 \\
 26 & TConv2d & 25 & 14x14x128 & 4x4 & 2 & 1 \\
 27 & TConv2d & 26 & 14x14x128 & 3x3 & 1 & 1 \\
 28 & TConv2d & 27 & 14x14x128 & 3x3 & 1 & 1 \\
 29 & TConv2d & 28 & 28x28x64 & 4x4 & 2 & 1 \\
 30 & TConv2d & 29 & 28x28x64 & 3x3 & 1 & 1 \\
 31 & TConv2d & 30 & 28x28x64 & 3x3 & 1 & 1 \\
 32 & TConv2d & 31 & 56x56x64 & 4x4 & 2 & 1 \\
 33 & TConv2d & 32 & 56x56x64 & 3x3 & 1 & 1 \\
 34 & TConv2d & 33 & 56x56x64 & 3x3 & 1 & 1 \\
 35 & TConv2d & 34 & 112x112x32 & 4x4 & 2 & 1 \\
 36 & TConv2d & 35 & 112x112x32 & 3x3 & 1 & 1 \\
 37 & TConv2d & 36 & 112x112x32 & 3x3 & 1 & 1 \\
 38 & TConv2d & 37 & 224x224x32 & 4x4 & 2 & 1 \\
 39 & TConv2d & 38 & 224x224x32 & 3x3 & 1 & 1 \\
 40 & TConv2d & 39 & 224x224x3 & 3x3 & 1 & 1 \\
 \end{tabular}
\end{center}
\end{table}

\begin{table}[h]
\begin{center}
 \caption{Network architecture for discriminator $D$. Except for the input and layer 5, each layer is followed by a batch normalization layer and ReLU activation. Layer 5 is followed by sigmoid activation function.}\vspace{1ex}
 \label{tab:d}
 \begin{tabular}{lllcccc}
 No. & Layer & Input & Output Size & Kernel & Stride & Padding \\ \hline 
 0 & Input & $\textbf{x}/\hat{\textbf{x}}+ \textbf{m}$ & 224x224x4 & & & \\ 
 1 & Conv2d & 0 & 112x112x64 & 4x4 & 2 & 1 \\
 2 & Conv2d & 1 & 56x56x128 & 4x4 & 2 & 1 \\
 3 & Conv2d & 2 & 28x28x256 & 4x4 & 2 & 1 \\
 4 & Conv2d & 3 & 14x14x512 & 4x4 & 2 & 1 \\
 5 & Conv2d & 4 & 1x1x1 & 14x14 & 1 & 0 \\
 \end{tabular}
\end{center}
\end{table}

\begin{table}[h]
\begin{center}
 \caption{Network architecture for \textit{PatchClass13}. Except for the input and layer 7, each layer is followed by a batch normalization layer and ReLU activation. RF stands for the maximum receptive field of a pixel in the output of the respective layer. TConv2d denotes transposed convolutional layers \cite{Zeiler2010}.}\vspace{1ex}
 \label{tab:patchdiff13}
 \begin{tabular}{lllccccc}
 No. & Layer & Input & Output Size & Kernel & Stride & Padding & RF\\ \hline 
 0 & Input & $\textbf{x}$ & 224x224x3 & & & & 1\\ 
 1 & Conv2d & 0 & 224x224x32 & 3x3 & 1 & 1 & 3\\
 2 & Conv2d & 1 & 224x224x32 & 3x3 & 1 & 1 & 5\\
 3 & Conv2d & 2 & 112x112x32 & 3x3 & 2 & 1 & 7\\
 4 & TConv2d & 3 & 224x224x32 & 3x3 & 2 & 1 & 9\\
 5 & TConv2d & 4 & 224x224x32 & 3x3 & 1 & 1 & 11\\
 6 & TConv2d & 5 & 224x224x32 & 3x3 & 1 & 1 & 13\\
 7 & Conv2d & 6 & 224x224x2 & 1x1 & 1 & 1 & 13\\
 \end{tabular}
\end{center}
\end{table}

\begin{table}[h]
\begin{center}
 \caption{Network architecture for \textit{PatchClass21}. Except for the input and layer 9, each layer is followed by a batch normalization layer and ReLU activation. RF stands for the maximum receptive field of a pixel in the output of the respective layer. TConv2d denotes transposed convolutional layers.}\vspace{1ex}
 \label{tab:patchdiff21}
 \begin{tabular}{lllccccc}
 No. & Layer & Input & Output Size & Kernel & Stride & Padding & RF\\ \hline 
 0 & Input & $\textbf{x}$ & 224x224x3 & & & & 1\\ 
 1 & Conv2d & 0 & 224x224x32 & 3x3 & 1 & 1 & 3\\
 2 & Conv2d & 1 & 224x224x32 & 3x3 & 1 & 1 & 5\\
 3 & Conv2d & 2 & 112x112x32 & 3x3 & 2 & 1 & 7\\
 4 & Conv2d & 3 & 112x112x64 & 3x3 & 1 & 1 & 11\\
 5 & TConv2d & 4 & 112x112x32 & 3x3 & 1 & 1 & 15\\
 6 & TConv2d & 5 & 224x224x32 & 3x3 & 2 & 1 & 17 \\
 7 & TConv2d & 2 + 6& 224x224x32 & 3x3 & 1 & 1 & 19 \\
 8 & TConv2d & 7 & 224x224x32 & 3x3 & 1 & 1 & 21\\
 9 & Conv2d & 8 & 224x224x2 & 1x1 & 1 & 1 & 21\\
 \end{tabular}
\end{center}
\end{table}

\begin{table}[h]
\begin{center}
 \caption{Network architecture for \textit{PatchClass29}. Except for the input and layer 11, each layer is followed by a batch normalization layer and ReLU activation. RF stands for the maximum receptive field of a pixel in the output of the respective layer. TConv2d denotes transposed convolutional layers.}\vspace{1ex}
 \label{tab:patchdiff29}
 \begin{tabular}{lllccccc}
 No. & Layer & Input & Output Size & Kernel & Stride & Padding & RF\\ \hline 
 0 & Input & $\textbf{x}$ & 224x224x3 & & & & 1\\ 
 1 & Conv2d & 0 & 224x224x32 & 3x3 & 1 & 1 & 3\\
 2 & Conv2d & 1 & 224x224x32 & 3x3 & 1 & 1 & 5\\
 3 & Conv2d & 2 & 112x112x32 & 3x3 & 2 & 1 & 7\\
 4 & Conv2d & 3 & 112x112x64 & 3x3 & 1 & 1 & 11\\
 5 & Conv2d & 4 & 112x112x64 & 3x3 & 1 & 1 & 15\\
 6 & TConv2d & 5 & 112x112x64 & 3x3 & 1 & 1 & 19\\
 7 & TConv2d & 6 & 112x112x32 & 3x3 & 1 & 1 & 23\\
 8 & TConv2d & 7 & 224x224x32 & 3x3 & 2 & 1 & 25 \\
 9 & TConv2d & 2 + 8& 224x224x32 & 3x3 & 1 & 1 & 27\\
 10 & TConv2d & 9 & 224x224x32 & 3x3 & 1 & 1 & 29\\
 11 & Conv2d & 10 & 224x224x2 & 1x1 & 1 & 1 & 29\\
 \end{tabular}
\end{center}
\end{table}

\begin{table}[h]
\begin{center}
 \caption{Network architecture for \textit{PatchClass35}. Except for the input and layer 13, each layer is followed by a batch normalization layer and ReLU activation. RF stands for the maximum receptive field of a pixel in the output of the respective layer. TConv2d denotes transposed convolutional layers.}\vspace{1ex}
 \label{tab:patchdiff35}
 \begin{tabular}{lllccccc}
 No. & Layer & Input & Output Size & Kernel & Stride & Padding & RF \\ \hline 
 0 & Input & $\textbf{x}$ & 224x224x3 & & & & 1\\ 
 1 & Conv2d & 0 & 224x224x32 & 3x3 & 1 & 1 & 3\\
 2 & Conv2d & 1 & 224x224x32 & 3x3 & 1 & 1 & 5\\
 3 & Conv2d & 2 & 112x112x32 & 3x3 & 2 & 1 & 7\\
 4 & Conv2d & 3 & 112x112x64 & 3x3 & 1 & 1 & 11\\
 5 & Conv2d & 4 & 112x112x64 & 3x3 & 1 & 1 & 15\\
 6 & Conv2d & 5 & 56x56x64 & 3x3 & 2 & 1 & 19\\
 7 & TConv2d & 6 & 112x112x64 & 3x3 & 2 & 1 & 23 \\
 8 & TConv2d & 5 + 7 & 112x112x64 & 3x3 & 1 & 1 & 27\\
 9 & TConv2d & 8 & 112x112x32 & 3x3 & 1 & 1 & 31 \\
 10 & TConv2d & 9 & 224x224x32 & 3x3 & 2 & 1 & 31 \\
 11 & TConv2d & 2 + 10& 224x224x32 & 3x3 & 1 & 1 & 35 \\
 12 & TConv2d & 11 & 224x224x32 & 3x3 & 1 & 1 & 35 \\
 13 & Conv2d & 12 & 224x224x2 & 1x1 & 1 & 1 & 35 \\
 \end{tabular}
\end{center}
\end{table}

\begin{table}[h]
\begin{center}
 \caption{Network architecture for \textit{PatchClass51}. Except for the input and layer 15, each layer is followed by a batch normalization layer and ReLU activation. RF stands for the maximum receptive field of a pixel in the output of the respective layer. TConv2d denotes transposed convolutional layers.}\vspace{1ex}
 \label{tab:patchdiff51}
 \begin{tabular}{lllccccc}
 No. & Layer & Input & Output Size & Kernel & Stride & Padding & RF\\ \hline 
 0 & Input & $\textbf{x}$ & 224x224x3 & & & & 1\\ 
 1 & Conv2d & 0 & 224x224x32 & 3x3 & 1 & 1 & 3\\
 2 & Conv2d & 1 & 224x224x32 & 3x3 & 1 & 1 & 5\\
 3 & Conv2d & 2 & 112x112x32 & 3x3 & 2 & 1 & 7\\
 4 & Conv2d & 3 & 112x112x64 & 3x3 & 1 & 1 & 11\\
 5 & Conv2d & 4 & 112x112x64 & 3x3 & 1 & 1 & 15\\
 6 & Conv2d & 5 & 56x56x64 & 3x3 & 2 & 1 & 19\\
 7 & Conv2d & 6 & 56x56x128 & 3x3 & 1 & 1 & 27\\
 8 & TConv2d & 7 & 56x56x64 & 3x3 & 1 & 1 & 35\\
 9 & TConv2d & 8 & 112x112x64 & 3x3 & 2 & 1 & 39 \\
 10 & TConv2d & 5 + 9 & 112x112x64 & 3x3 & 1 & 1 & 43\\
 11 & TConv2d & 10 & 112x112x32 & 3x3 & 1 & 1 & 47 \\
 12 & TConv2d & 11 & 224x224x32 & 3x3 & 2 & 1 & 47\\
 13 & TConv2d & 2 + 12& 224x224x32 & 3x3 & 1 & 1 & 51\\
 14 & TConv2d & 13 & 224x224x32 & 3x3 & 1 & 1 & 51\\
 15 & Conv2d & 14 & 224x224x2 & 1x1 & 1 & 1 & 51 \\
 \end{tabular}
\end{center}
\end{table}
